# Supplementary material for: AfriNames: Most ASR models "butcher" African Names
Source: arXiv:2306.00253 source file (2023-06-02)
Supplement: Supplementary file 1 [file appendix.tex]

% Appendix
\onecolumn
\appendix
\section{Appendix}
%You may include other additional sections here.
\begin{table}[h]
    \caption{Examples using our best (fine-tuned) model, Whisper-Medium-General, showing samples with WER $>$ 0.8 on the pre-trained whisper model}

    \tiny
    \centering
    \begin{tabular}{p{1cm}p{1cm}p{1cm}p{2.3cm}p{2.3cm}p{1cm}p{2.3cm}p{1cm}}
% \begin{tabular}{lllllrlr}
\toprule
PER &   LOC &  ORG &  Reference & Prediction Pre-trained &  WER Pretrained & Prediction Fine-tune &  WER Fine-tune \\
\midrule
% tinubu & - & - & tinubu as a game-master in politics can sacrifice personal interests for his partys win. & tanubu as a keymaster in politicians and surprise personnel in stressful responses, when in first-order. & 0.857 & tinubu as a game-master in politics can sacrifice personal interests for his partys win. & 0.000 \\
% \hline
\colorbox{yellow}{daberechi}, \colorbox{yellow}{iniola} & - & - & dr \colorbox{yellow}{daberechi} neonatal intensive care unit (icu) aware and dr \colorbox{yellow}{iniola} surgery notified. 09 january, 2003 & dr. \colorbox{yellow}{davirechi} nyunato, intensive care unit, awuya, and dr. \colorbox{yellow}{inuyo} la sajar, notified 9th january, 2003. & 0.813 & dr \colorbox{yellow}{daberechi} neonatal intensive care unit (icu) and dr \colorbox{yellow}{inyola} surgery notified. 09 jan, 2003 & 0.188 \\
\hline
uloaku, onyinyechukwu, ne, ice finidi & - & - & dr. uloaku is w/ the pt onyinyechukwu at this time and has also spoken to pt's neice finidi & the other first of uno aco is w- the patient on iyukchuku at the time and has also spoken to patient apostrophe s, ms. findi. & 0.889 & dr. nnuaku is w/ the pt onyinyechukwu at the time and has also spoken to pt's neice tinde & 0.167 \\
\hline
udeme obong, abiona & ikeja & - & udeme obong will be in to visit abiona in the am at ikeja & in 2 days, ubuntu will be introduced in the am or tk job. & 0.846 & udimi obong will be in to visit obiona in the am for thickly joe & 0.385 \\
\hline
\colorbox{yellow}{zeribe} & - & - & patient zeribe presented on account of ammenorrhea of 4 months. next line. hot flushes associated with night sweats & patient \colorbox{yellow}{0} will be represented on a count of arm and ear of a 4-month-old. next line. outflotches are associated with 9th sweat. & 0.833 & patient \colorbox{yellow}{zirinbe} presented on account of ammenorrhea of 4 months. next line. hot flushes associated with night sweats & 0.0556 \\
\hline
ubanwa ibimina, kasiemobi & - & - & thu 04 feb, 1988 ob: dr. ubanwa ibimina dr. kasiemobi & thursday, 4th february, 1988, obi-kolun, dr. ubangwa ibimina, dr. kasiem obi, & 0.900 & thursday 04 february, 1988 ob: dr. obanwa ibimina dr. kasiemobi & 0.300 \\
\hline
ogechukwukana, mahaja onyedikachukwu & birnin kebbi & - & ogechukwukana has been living at birnin kebbi with his wife mahaja onyedikachukwu who helps with his medications. & so, & 1.000 & ogichukwukana has been living at birnin kebbi with his wife mahaja oyedikachukwu who helps with his medications. & 0.118 \\
\hline
\colorbox{yellow}{chiehidra nkediniruka}, \colorbox{yellow}{obi} & - & \colorbox{yellow}{warri} & top gynecologists, drs \colorbox{yellow}{chiehidra nkediniruka} and \colorbox{yellow}{obi} at \colorbox{yellow}{warri} leading specialist hospital were quizzed on the management of several patients. & i'm a college is common that does she i'd rather in getting a little bit for really in specialist hospital yes kids on the management of several patients who stop & 1.150 & top gynecologists, drs \colorbox{yellow}{chiehidra nketeenerewa} and \colorbox{yellow}{obi} at \colorbox{yellow}{warri} leading specialist hospital were skilled to the management of several patients. & 0.150 \\
\hline
ibiama', ayotola, nnennaya & potiskum & lekki clinic & patient's family members ibiama and ayotola showed up to the potiskum ward this morning looking for nnennaya who passed away last night at lekki clinic. & patient family members & 0.920 & patient's family members yabiamma and ayotola showed up to the potiskum ward this morning looking for nnennaya who passed away last night at 30 clinic. & 0.080 \\
\bottomrule
\end{tabular}
    \label{apdx:nigeria_ner2}
\end{table}

\begin{table}[h]
    \caption{Examples using our best (fine-tuned) model, Whisper-Medium-General, showing samples with WER $<$ 0.2 on the pre-trained whisper model}

    \tiny
    \centering
    \begin{tabular}{p{1cm}p{1cm}p{1cm}p{2.3cm}p{2.3cm}p{1cm}p{2.3cm}p{1cm}}
% \begin{tabular}{lllllrlr}
\toprule
PER &   LOC &  ORG &  Reference & Prediction Pre-trained &  WER Pretrained & Prediction Fine-tune &  WER Fine-tune \\
\midrule
\colorbox{yellow}{femi} & \colorbox{yellow}{nigeria} & - & \colorbox{yellow}{femi} says 21 not 18 persons have been killed in the first 14 days of the coronavirus lockdown in \colorbox{yellow}{nigeria} so far. & \colorbox{yellow}{phenyl} says 21 not 18 persons have been cured in the first 14 days of the coronavirus lockdown in \colorbox{yellow}{nigeria} so far. & 0.091 & \colorbox{yellow}{femi} says 21 not 18 persons have been killed in the first 14 days of the coronavirus lockdown in \colorbox{yellow}{nigeria} so far. & 0.000 \\
\hline
chinweizu Ojo, bu, kola & eket & - & children chinweizu ojo and bukola were found last night wandering the streets unattended after their mother and father, went missing while returning from work at eket & children chinweuzu, ojo and bukola were found last night wandering the streets unattended after their mother and father, went missing while returning from work at eket. & 0.077 & children chinweizu ojo and bukola were found last night wandering the streets unattended after their mother and father, went missing while returning from work at eket & 0.000 \\
\hline
N, nanna, Chimaihe & - & - & nnanna was watching tv as they normally do in the evening when his brother chimaihe went to prepare dinner. & nana was watching tv as they normally do in the evening when his brother chimaehe went to prepare dinner. & 0.105 & nnanna was watching tv as they normally do in the evening when his brother chimaihe went to prepare dinner. & 0.000 \\
\hline
\colorbox{yellow}{femi} & - & - & the event, which lasted five hours, was also used as a platform to surprise \colorbox{yellow}{femi} with a rare saxophone as a birthday gift before he sets out on his seven-week american tour. & the event, which lasted five hours, was also used as a platform to surprise \colorbox{yellow}{femi} with a real saxophone as a birthday gift before it set out on a seven-week american tour. & 0.125 & the event, which lasted five hours, was also used as a platform to surprise \colorbox{yellow}{femi} with a rare saxophone as a birthday gift before he sets out on his seven week american tour. & 0.0625 \\
\hline
akubuilo & - & umuahia elementary school & akubuilo began playing the piano when he was a young child at umuahia elementary school & akubuilo began playing the piano when he was a young child at omuahe elementary school. & 0.133 & acobuilo began playing the piano when he was a young child at omuahia elementary school & 0.133 \\
\hline
kilani & - & asaba elementary school & kilani began playing the piano when he was a young child at asaba elementary school & killani began playing the piano when he was a young child at asaba elementary school. & 0.133 & kilani began playing the piano when he was a young child at asaba elementary school & 0.000 \\
\hline
\colorbox{yellow}{ihuoma}, \colorbox{yellow}{inango} & - & - & patient \colorbox{yellow}{ihuoma} was addicted to morphine and eventually had to see dr. \colorbox{yellow}{inango} & patient \colorbox{yellow}{ioma} was addicted to morphine and eventually had to see dr. \colorbox{yellow}{enango}. & 0.154 & patient \colorbox{yellow}{ihuoma} was addicted to morphine and eventually had to see dr. \colorbox{yellow}{inango} & 0.000 \\
\hline
ojo & jordan & nigerian tribune & speaking with the nigerian tribune on the significance of jordan to the christian faithful, prophet ojo described it as a land of separation from the land of reproach to that of promise. & speaking with the nigerian tribune on the significance of jordan to the christian faithful, prophet ojo described it as a land of separation from the land of reproach to that of promise. & 0.000 & speaking with the nigerian tribune on the significance of jordan to the christian faithful, prophet ojoe described it as a land of separation from the land of rep ridge to that of promise. & 0.0938 \\
\bottomrule
\end{tabular}
    \label{apdx:nigeria_ner1}
\end{table}

\begin{figure}[H]
\includegraphics[scale=0.3]{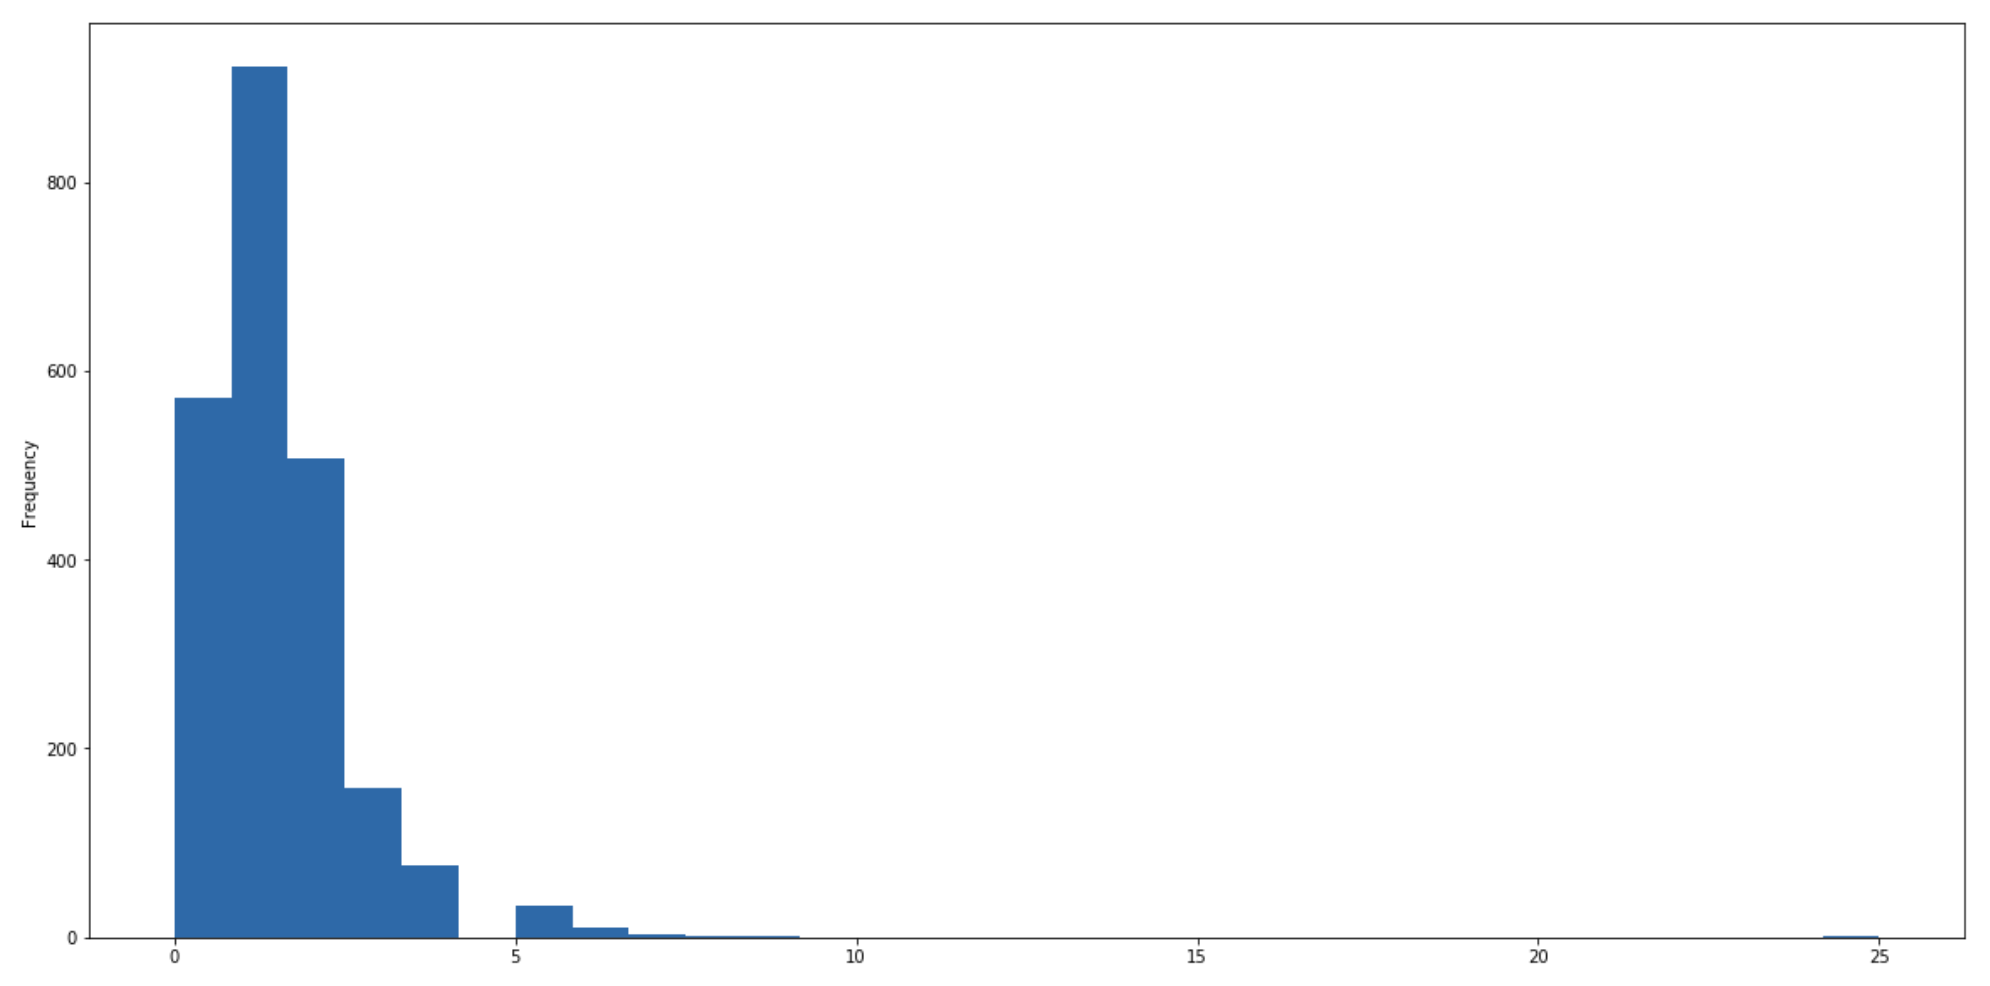} %
\centering
\caption{Distribution of named entities in AfriSpeech test partition}
\label{fig:distribution}
\end{figure}
